# Supplementary material for: Weakly Supervised Contrastive Learning for Chest X-Ray Report Generation
Source: arXiv:2109.12242 source file (2021-09-25)
Supplement: Supplementary file 1 [file supple.tex]

\appendix

\section{Appendices}
\paragraph{Generated samples}
We show some generated samples from MIMIC-ABN and MIMIC-CXR in
\cref{tab:abn-samples} and \cref{tab:cxr-samples}.

\begin{table*}[t]
\small
\centering
\setlength{\tabcolsep}{2pt}
% \resizebox{\linewidth}{!}{
\begin{tabular}{p{0.9\textwidth} }
\toprule
\textbf{GT}: low lung volumes exaggerate the cardiac size which may still be enlarged as well as contribute to minimal basilar atelectasis. chest radiography is nonsensitive for bony abnormalities and dedicated views should be obtained if indicated. \\
\textbf{WCL}: lung volumes are low. heart size is accentuated as. result appearing borderline enlarged. apart from subsegmental atelectasis in the lung bases the lungs are clear without focal consolidation. low lung volumes without focal consolidation. \\
\midrule 
\textbf{GT}: streaky left basilar opacity likely reflects atelectasis. minimal left basilar atelectasis. history. with history of myocardial infarction presenting with epigastric pain. \\
\textbf{WCL}: linear left basilar opacity is likely atelectasis versus scarring. m with chest pain.\\
\midrule 
\textbf{GT}: the lungs are hyperexpanded but clear consolidation effusion or pneumothorax. increased lucency at the left lung apex and linear markings on the lateral raises the possibility apical bullous disease. hyperexpansion without acute cardiopulmonary process. \\
\textbf{WCL}: the lungs are hyperinflated but clear of consolidation or effusion. hyperinflation without acute cardiopulmonary process. \\
\midrule 
\textbf{GT}: there is bibasilar atelectasis. a linq cardiac monitoring device projects over the subcutaneous tissue of the left lower chest. f with shortness of breath. evaluate for pneumonia. \\
\textbf{WCL}: the lungs are hyperinflated with flattening of the diaphragms suggesting chronic obstructive pulmonary disease. there is mild bibasilar atelectasis. \\
\midrule 
\textbf{GT}: there is. subtle opacity in the right upper lobe projecting just above the minor fissure compatible with pneumonia. cervical spinal hardware in the lower cervical spine is noted. findings concerning for pneumonia in the right upper lobe. followup to resolution advised. \\
\textbf{WCL}: right chest wall port is seen with catheter tip in the upper right atrium. linear right basilar opacity is likely atelectasis. cardiac silhouette is mildly enlarged. atherosclerotic calcifications noted at the aortic arch. mild cardiomegaly. right basilar opacity potentially atelectasis noting that infection is not entirely excluded. f with fever on chemo ro acute infectious process. \\
\midrule 
\textbf{GT}: the lung volumes are low. severe scoliosis of the thoracic spine with subsequent asymmetry of the ribcage. year old woman with increased dyspnea dementia dysphagia. at risk aspiration. non-focal clinical exam  evaluate for abnormalities. \\
\textbf{WCL}: in comparison with the study of there is little change and no evidence of acute cardiopulmonary disease. continued elevation of the left hemidiaphragm. \\

\midrule 
\textbf{GT}: linear atelectasis is noted at the left lung base and right midlung. -year-old female with chest pain. evaluate for acute cardiopulmonary process. \\
\textbf{WCL}: linear opacity at the left lung base is most suggestive of atelectasis and is unchanged. f with chest pain ro pneumothorax.\\
\midrule 
\textbf{GT}: the lung volumes are low and the lungs are clear of focal consolidation or edema. the heart continues to be enlarged. a right port-a-cath terminates at the cavoatrial junction. there is pneumoperitoneum better seen on the abdominal ct scan. pneumoperitoneum. history. with bilateral crackles fever  evaluate for acute process. \\
\textbf{WCL}: there is. left lower lobe retrocardiac opacity better delineated on ct from the same day. there is. left lower lobe opacity better assessed on ct from the same day. there is mild left basal atelectasis. there is pulmonary vascular congestion. left lower lobe retrocardiac opacity better assessed on ct from the same day. likely pulmonary vascular congestion\\
\bottomrule
\end{tabular}
\caption{Generated samples from MIMIC-ABN dataset.
}
\label{tab:abn-samples}
\end{table*}

\begin{table*}[t]
\small
\centering
\setlength{\tabcolsep}{2pt}
% \resizebox{\linewidth}{!}{
\begin{tabular}{p{0.9\textwidth} }
\toprule
\textbf{GT}: there is moderate amount of right-sided subcutaneous emphysema which is similar in appearance compared to prior. right-sided chest tube is again visualized. there is no increase in the pneumothorax. bilateral parenchymal opacities are again visualized and not significantly changed. the tracheostomy tube is in standard location. right subclavian line tip is in the mid svc.
\\
\textbf{WCL}: tracheostomy tube tip is in unchanged position. right-sided port-a-cath tip terminates in the low svc. left-sided port-a-cath tip terminates in the proximal right atrium unchanged. heart size is normal. mediastinal and hilar contours are similar. innumerable bilateral pulmonary nodules are re- demonstrated better assessed on the previous ct. small right pleural effusion appears slightly increased compared to the prior exam. small left pleural effusion is similar. no new focal consolidation or pneumothorax is present. there are no acute osseous abnormalities.\\
\midrule 
\textbf{GT}: a large-bore central catheter terminates in the expected location of the right atrium unchanged from prior. the lungs are clear. there is no focal consolidation or pneumothorax. there is no vascular congestion or pleural effusions. mediastinal and hilar contours are within normal limits. the cardiac silhouette is mildly enlarged though unchanged. mild indentation of the left trachea at the level of the clavicles is unchanged compared to prior chest ct from  and likely reflects an underlying tracheal deformity as no compressive mass lesion is evident on the prior ct. \\
\textbf{WCL}: pa and lateral views of the chest provided. dialysis catheter is unchanged with tip extending to the region of the low svc. the heart remains mildly enlarged. there is hilar congestion and mild interstitial pulmonary edema. no large effusion or pneumothorax. bony structures are intact. \\
\midrule 
\textbf{GT}: the lungs are mildly hyperinflated as evidenced by flattening of the diaphragms on the lateral view. diffuse interstitial markings compatible with known chronic interstitial lung disease are unchanged. there is no pleural effusion or evidence of pulmonary edema. there is no focal airspace consolidation worrisome for pneumonia. mild to moderate cardiomegaly is unchanged. the mediastinal and hilar contours are unremarkable. a coronary artery stent is noted. there is. levoscoliosis of the thoracic spine . \\
\textbf{WCL}: lung volumes are low. heart size is mildly enlarged. the aorta is tortuous and diffusely calcified. crowding of bronchovascular structures is present without overt pulmonary edema. patchy opacities in the lung bases likely reflect areas of atelectasis. no focal consolidation pleural effusion or pneumothorax is present. there are no acute osseous abnormalities.\\
\midrule 
\textbf{GT}: as compared to the previous radiograph there is no relevant change. no definite proof of pneumonia. unchanged borderline size of the cardiac silhouette without evidence of overt pulmonary edema. minimal atelectasis at the left lung base and minimal bilateral pleural effusions restricted to the dorsal costophrenic sinuses better appreciated on the lateral than on the frontal radiograph. known skeletal changes. \\
\textbf{WCL}: as compared to the previous radiograph there is. newly appeared parenchymal opacity at the right lung base. the opacity is ill-defined and shows air bronchograms. in the appropriate clinical setting these changes are highly suggestive of pneumonia. at the time of dictation and observation <unk> am on the referring physician. was paged for notification. otherwise the radiograph is unchanged. the findings were subsequently discussed over the telephone.\\

\midrule 
\textbf{GT}: frontal and lateral views of the chest were obtained. the patient is status post median sternotomy and cabg. left-sided aicd is unchanged in position. patchy right lower lobe opacity is seen worrisome for consolidation which could be due to infection or aspiration. no pleural effusion or pneumothorax is seen. the cardiac and mediastinal silhouettes are stable with the cardiac silhouette top normal. \\
\textbf{WCL}: single portable view of the chest is compared to previous exam from. when compared to prior there has been no significant interval change. again seen is mild pulmonary vascular congestion. blunting of the lateral costophrenic angles could be due to small effusions. cardiac silhouette is enlarged but stable. dual-lead pacing device is again seen with lead tips in the right atrium and right ventricle. osseous and soft tissue structures are unchanged. \\
\bottomrule
\end{tabular}
\caption{Generated samples from MIMIC-CXR dataset.
}
\label{tab:cxr-samples}
\end{table*}

\paragraph{More implementation details:}
Our models are trained on a Linux server with Quadro RTX 8000. 
The number of parameters for our full model is 82.53 million. 
All models are trained with 30 epochs. 
The average time for training is around 10 hours for MIMIC-ABN and 30 hours for MIMIC-CXR. 
We conduct a grid-based hyperparameter search for weighting factor $\lambda \in \{0.1, 0.2, 0.3, 0.4, 0.5\}$ and temperature $\tau \in \{0.1, 1, 10\}$ by evaluating the models on the validation sets of the two datasets. 
Words with frequency less than 3 times are disregarded for MIMIC-ABN and 10 times for MIMIC-CXR.
The maximum sequence lengths are set to 64 and 100 for MIMIC-ABN and MIMIC-CXR. 
The projection heads consists of two convolutional layers with ReLU activation, and the latent dimensions are set to 256 for both visual and text projection layers.
The number of heads in the transformer is 8. Both encoder and decoder consists of 3 self-attention layers.
